# Supplementary material for: Tree-based Implementation of the Small Matrix Path Integral for System-Bath Dynamics
Source: arXiv:2207.11830 source file (2023-12-10)
Supplement: Supplementary file 1 [file appendix.tex]

\newpage
\section*{Appendix}
\begin{figure}[h!]
\begin{center}
\begin{tabular}{c|c c c c c c}
    & $k=0$ & $k=1$ & $k=2$ & $k=3$ & $k=4$ & $\dots$ \\ \hline
    $n=0$ & 0 &  \\
    $n=1$ & 1 & 0  \\
    $n=2$ & 3 & 2 & 0 \\
    $n=3$ & 6 & 9 & 7 & 0 \\
    $n=4$ & 10 & 24 & 32 & 27 & 0 \\
    $\vdots$ & $\vdots$ & $\vdots$ & $\vdots$ & $\vdots$ & $\vdots$ & $\ddots$
\end{tabular}
\end{center}
    \caption{First five rows of the triangle $S(n,k)$.}
    \label{fig_S}
\end{figure}

Boundary values
\begin{equation*}
    S(n,n) = 0
\end{equation*}
for $n=0,2\dots$.
\begin{equation}
    \label{Eq_1}
    S(n,k) = \sum_{j=0}^{k} S(n-1,j) + \frac{(n-k)^2}{n} \binom{n-1+k}{k}
\end{equation}
for $n=1,2,\dots$, $k=0,\cdots,n-1$.
In particular,
\begin{equation*}
    S(n,0) = S(n-1,0) + n
\end{equation*}
indicates that
\begin{equation*}
    S(n,0) = \frac{n(n+1)}{2}.
\end{equation*}
Assume
\begin{equation*}
    f(x,y) = \sum_{n=0}^{\infty} \sum_{k=0}^{n} S(n,k) x^n y^k.
\end{equation*}
When $n=1,2,\dots$ and $k=1,\cdots,n-1$:
\begin{equation}
    \label{Eq_2}
    S(n,k-1) = \sum_{j=0}^{k-1} S(n-1,j) + \frac{(n-k+1)^2}{n} \binom{n+k-2}{k-1}.
\end{equation}
Take the difference of \cref{Eq_1,Eq_2},
 when $k=1,\dots,n-1$:
\begin{equation*}
    S(n,k) - S(n,k-1) = S(n-1,k) + \frac{\left[n^3-(2k+1)n^2+k^2n+k^2-k\right](n+k-2)!}{n!k!}
\end{equation*}
Multiply $x^n$, take sum for $n=1,2,\dots$ and $k=1,\dots,n-1$:
\begin{equation*}
\begin{split}
    &\sum_{n=1}^{\infty} \sum_{k=1}^{n-1}S(n,k) x^n
    - \sum_{n=1}^{\infty} \sum_{k=1}^{n-1} S(n,k-1) x^n \\
    =& \sum_{n=1}^{\infty} \sum_{k=1}^{n-1} S(n-1,k) x^n + 
    \frac{1-\sqrt{1-4x}-4x+2x\sqrt{1-4x} +x^2 - x^2\sqrt{1-4x}}{2(x-1)^2}
\end{split}
\end{equation*}
\ki{Cannot move on from here. The pattern of the off-diagonal sequence is unclear.}
\ki{In addition, our estimation may be kind of ``unfair'' as SMatPI can utilize the form of the triangle and use something similar to Qin Jiushao's algorithm to accelerate the computation. So I suggest to only put a lower bound of the SMatPI,
 which is still significantly larger than ours.}
